# Supplementary material for: Spontaneous lattice distortion and crystal field effects in HoB4
Source: arXiv:2510.01075 source file (2025-10-03)
Supplement: Supplementary file 1 [file SM.tex]

\documentclass[aps,prb,superscriptaddress,showpacs]{revtex4-1}
\usepackage{graphicx,bm,color,float,textcomp,mathtools,times,nicefrac}
\usepackage{subcaption}
\newcommand\HoB{HoB$_4$}

\usepackage{soul,xcolor}
\setstcolor{magenta}

\begin{document}

\renewcommand{\thefigure}{S\arabic{figure}}
\renewcommand{\thetable}{S\arabic{table}}
\renewcommand{\theequation}{S\arabic{equation}}

\makeatletter
\renewcommand\@bibitem[1]{\item\if@filesw \immediate\write\@auxout
    {\string\bibcite{#1}{S\the\value{\@listctr}}}\fi\ignorespaces}% <------------
\def\@biblabel#1{[S#1]}% <-------------------
\makeatother

\date{\today}
\title{Supplemental Material to ``Spontaneous lattice distortion and crystal field effects in HoB$_4$''}
\author{S.~Goswami}
\affiliation{Institute of Physics of the Czech Academy of Sciences, Na Slovance 2, 18200 Prague, Czech Republic}
\author{D. I.~Gorbunov}
\affiliation{Hochfeld-Magnetlabor Dresden (HLD-EMFL) and W\"urzburg-Dresden Cluster of Excellence ct.qmat, Helmholtz-Zentrum Dresden-Rossendorf, 01328 Dresden, Germany}
\author{D.~Kriegner}
\affiliation{Institute of Physics of the Czech Academy of Sciences, Na Slovance 2, 18200 Prague, Czech Republic}
\affiliation{Department of Condensed Matter Physics, Charles University, Ke Karlovu 5, 12116 Prague, Czech Republic}
\author{I.~Ishii}
\affiliation{Department of Quantum Matter, AdSE, Hiroshima University, Higashi-Hiroshima 739-8530, Japan}
\author{C. A.~Corr\^ea}
\affiliation{Institute of Physics of the Czech Academy of Sciences, Na Slovance 2, 18200 Prague, Czech Republic}
\author{T. Suzuki}
\affiliation{Department of Quantum Matter, AdSE, Hiroshima University, Higashi-Hiroshima 739-8530, Japan}
\author{D.~Brunt}
\affiliation{Department of Physics, University of Warwick, Coventry CV4 7AL, United Kingdom}
\affiliation{National Physical Laboratory, Hampton Road, Teddington TW11 0LW, United Kingdom}
\author{G.~Balakrishnan}
\affiliation{Department of Physics, University of Warwick, Coventry CV4 7AL, United Kingdom}
\author{S.~Zherlitsyn}
\affiliation{Hochfeld-Magnetlabor Dresden (HLD-EMFL), Helmholtz-Zentrum Dresden-Rossendorf, 01328 Dresden, Germany}
\author{J.~Wosnitza}
\affiliation{Hochfeld-Magnetlabor Dresden (HLD-EMFL), Helmholtz-Zentrum Dresden-Rossendorf, 01328 Dresden, Germany}
\affiliation{Institut fur Festk\"orper- und Materialphysik, TU Dresden, 01062 Dresden, Germany}
\author{O. A.~Petrenko}
\affiliation{Department of Physics, University of Warwick, Coventry CV4 7AL, United Kingdom}
\author{M. S.~Henriques}
\affiliation{Institute of Physics of the Czech Academy of Sciences, Na Slovance 2, 18200 Prague, Czech Republic}

\maketitle
%_________________________________________________________________________________________________
\subsection{Low-Temperature X-ray diffraction}

Additional results from the analysis of the low-temperature XRD (cooling) data of \HoB are presented here. They encompass the temperature evolution of selected peaks, fitting and deconvolution for the different symmetries, and the comparison of the lattice parameters on cooling and heating across the magnetic phase transitions.

%----- FIGURE 1 ------------------------------------------
\begin{figure*}[tb]
\includegraphics[width=0.99\columnwidth]{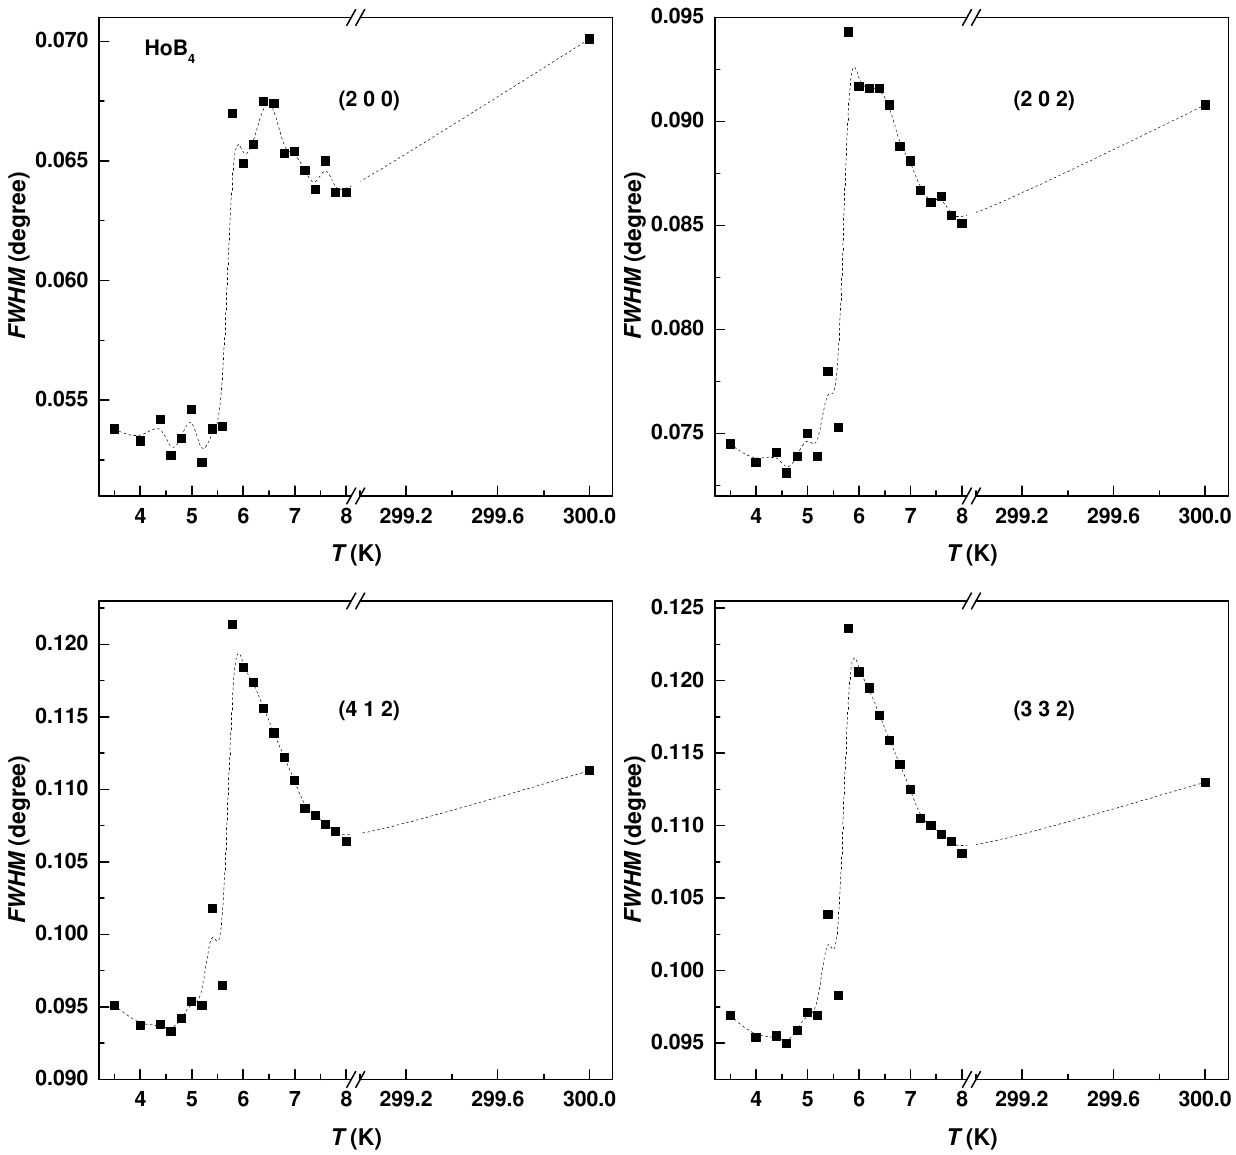}
\caption{Evolution of the FWHM of selected reflections with temperature in \HoB\ upon cooling.
The broken lines are guides to the eye.}
\label{fig:label1}
\end{figure*}

%----- FIGURE 2 ------------------------------------------
\begin{figure*}[tb]
\includegraphics[width=0.99\columnwidth]{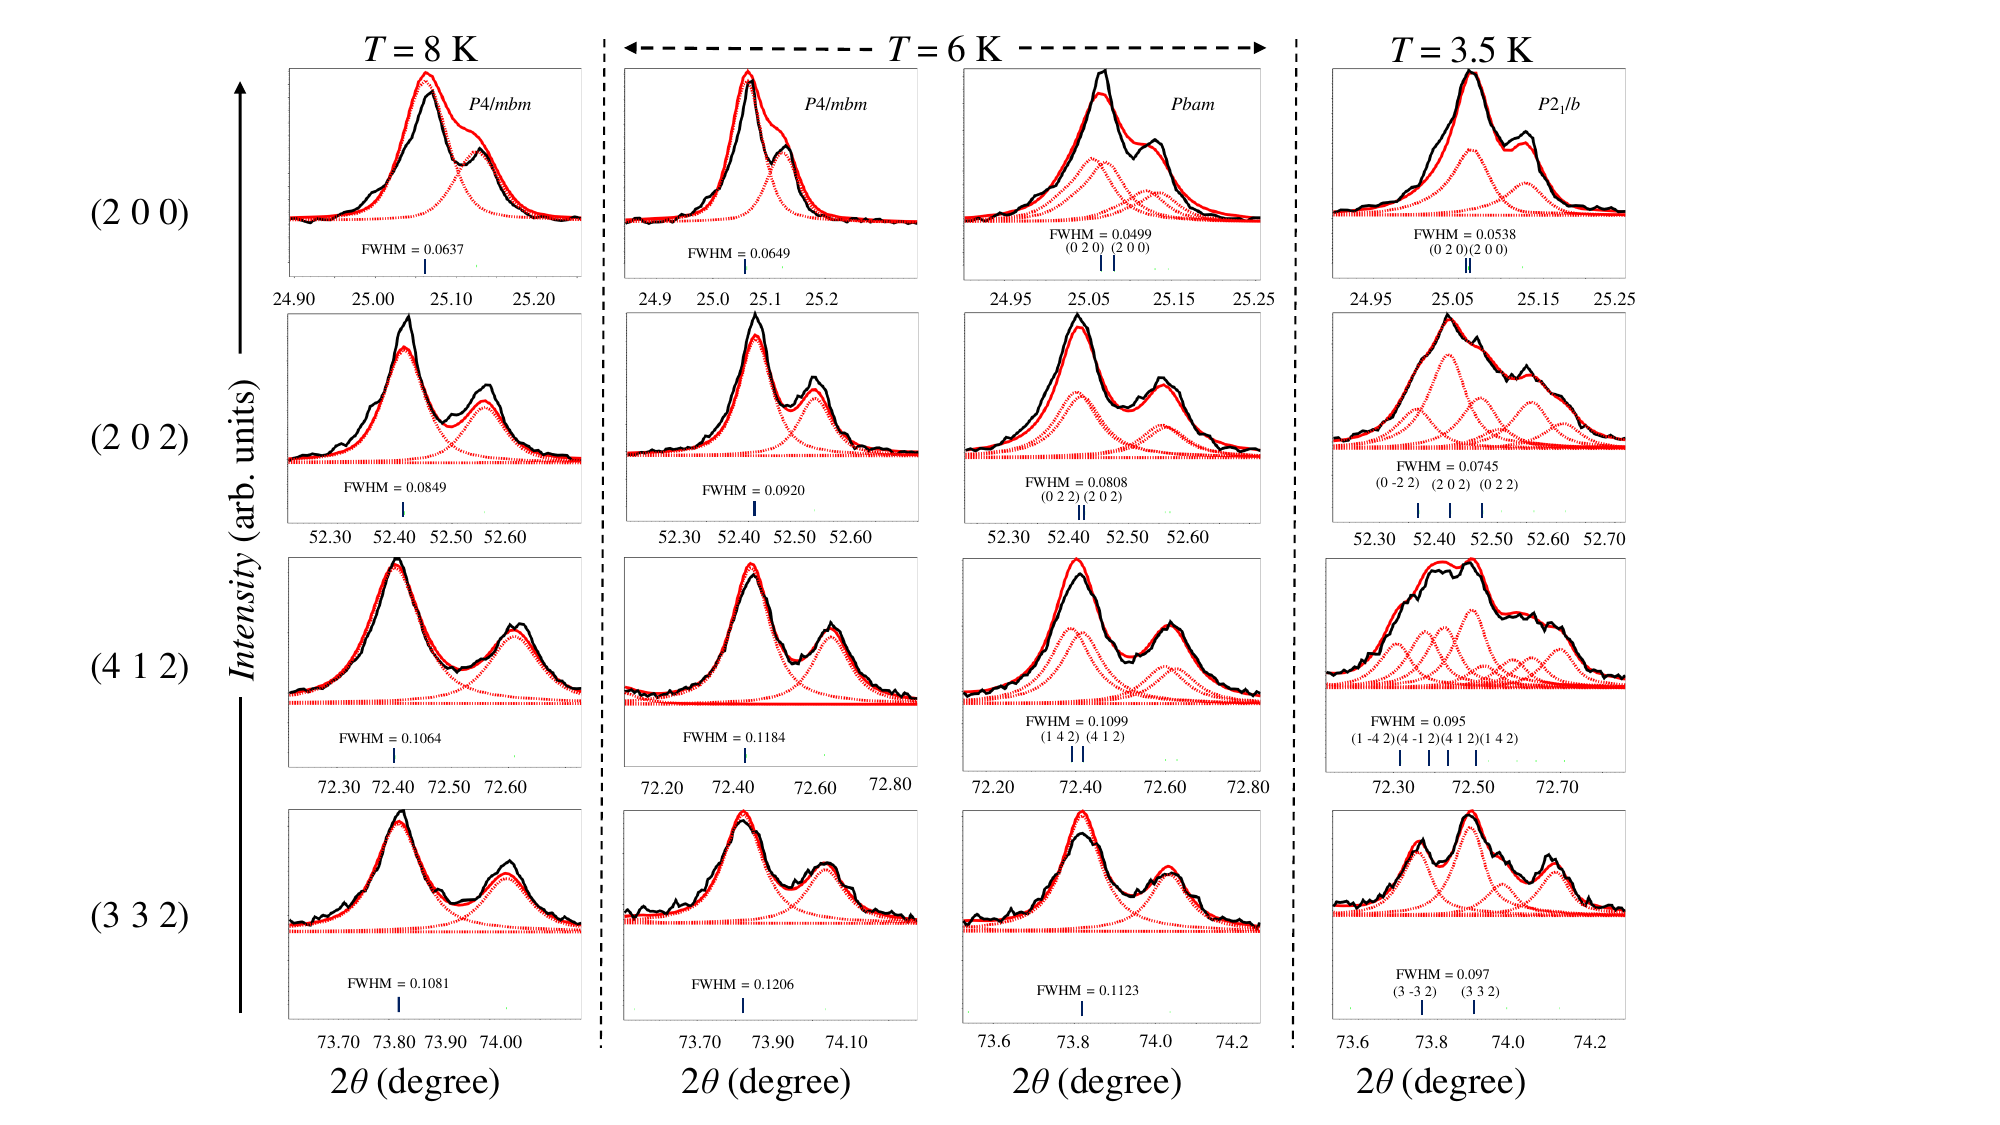}
\caption{Fitting curves (solid red line) to the XRD experimental cooling data (black line) and respective peak deconvolution (dashed red line) for the tetragonal and monoclinic space groups at 8~K and 3.5~K, respectively. Comparison of the fittings performed for the data at \textit{T}=6~K considering tetragonal and orthorhombic space groups.}
\label{fig:label1}
\end{figure*}

%----- FIGURE 3 ------------------------------------------
\begin{figure*}[tb]
\includegraphics[width=0.7\columnwidth]{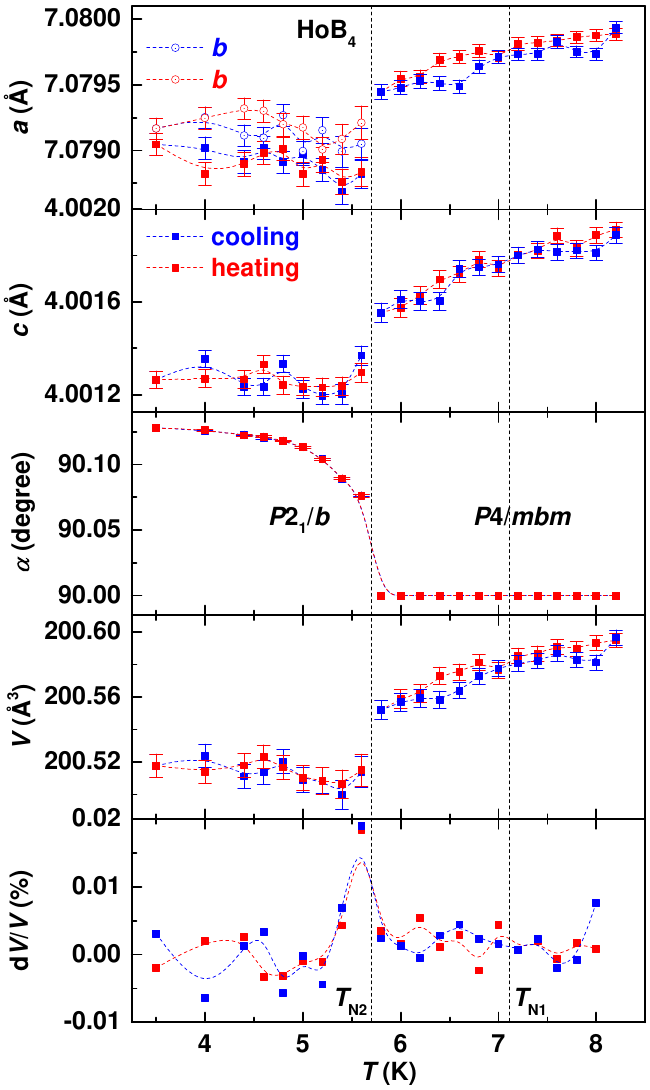}
\caption{Variation of lattice parameters, angle, unit cell volume, and volume changes with temperature for 8 K~$\ge T \ge$3.5~K in \HoB\ upon cooling and heating.
The broken lines are guides to the eye.}
\label{fig:label1}
\end{figure*} 

\bibliography{References_list} 
\end{document}
